# Supplementary material for: BreakBot: Analyzing the Impact of Breaking Changes to Assist Library Evolution
Source: arXiv:2111.05132 source file (2022-03-29)
Supplement: Supplementary file 1 [file appendix.tex]

\section{Comments}

\begin{itemize}[leftmargin=*]
	\item Don't forget it's double-blind (GitHub repositories, \etc)
\end{itemize}

Why do we need libraries?
\begin{itemize}[leftmargin=*]
	\item Software projects offer services and features target to meet user needs at a given point in time. This perceived benefit defines the value of the software artifact. 
	\item However, the environment, and user needs change over time, forcing projects to co-evolve in order to stay competitive. 
	\item The development of new functionality considered as part of the core services catalog of the project, entails the implementation of auxiliary utilities that do not add to the perceived worth of the product.
	\item Thus, the development of these extra features might negatively impact the project: changes entail additional costs and increase time to market, hindering its adoption by new users and severely impacting the value perception of old clients.
	\item To avoid this decrease in product value, library developers must find a way to cope with evolution. In particular, projects can depend on other projects offering the required features, to avoid incurring additional costs (mention other strategies to cope with change?). 
\end{itemize}

Software ecosystems and dependencies
\begin{itemize}[leftmargin=*]
	\item Some projects, therefore, assume the role of the dependee (a.k.a. libraries), and projects depending on such projects define themselves as dependants (a.k.a. clients).
	\item Progressively, interdependencies established among several projects sharing the same programming language, platform, or tools (Bogart, 2021) build up the backbone of a software ecosystem.
	\item However, the changing environment and the demands of the clients compels projects to consider incorporating new features, bug fixes, security patches, refactorings, or other types of changes responding to ripple effects (cyclic reasoning, already mentioned in the first part -> fix!).
\end{itemize}

Depending on the praised values, libraries can opt for any of the following evolution strategies:
\begin{enumerate}[leftmargin=*]
	\item impose burdensome costs on the client without incurring any cost as a library. 
Breaking changes are introduced without supporting clients; 
	\item mitigate costs on the client-side by investing some effort in assistance. 
Among possible techniques, libraries make an effort on communicating how to perform the upgrade or even include clients as part of their development process (Bogart, 2021), and; 
	\item assume all costs as a library alleviating costs on the client-side. 
For instance, libraries can maintain old interfaces, where deprecated elements coexist with new declarations. 
They can also uphold parallel releases, fixing bugs and security issues for a given major release even after newer major versions have been published (Bogart, 2021). 
However, technical debt is the cost to immobility: the library (and potentially its clients) reaches a point where its system is outdated or even obsolete.
\end{enumerate}

\begin{itemize}[leftmargin=*]
	\item The policies regarding software evolution, breaking changes, \etc differ largely from one ecosystem to the other (TOSEM'21), from one library to the other (Guava vs Apache vs \ldots), \etc $\rightarrow$ this meant BreakBot must make it possible to fine-tune the checking process according to one's policy (when/how to break, which clients, when to check and read the reports, \etc)
	\item Developers may leverage the information regarding breaking code in clients to (i)~prioritize information in their \texttt{CHANGELOG}, (ii)~suggest possible migrations according to typical usage, and even (iii)~open PRs on their clients' repositories to help them migrate (``\emph{forward impact management}'', De Souza and Redmiles)
	\item Highlight the notion of ``\emph{perception}?'' of the community:~might be right, might be wrong;~which influences decision-making;~need evidence-based decision-making instead
	\item Following TOSEM21's terminology, \emph{BB is a way to enforce values by implementing breaking change-related policies through tool-supported practices}!
	\item There is a \emph{cost} to immobility/stillness (\eg weird/bad names, old paradigms and interfaces, \etc), it scares people away! This immobility is due to strict policies regarding breaking changes. BB shall help developers preserve their attitude towards their values (\eg strong backward compatibility), while allowing them to make necessary changes \emph{when it is possible}.
	\item The absolute killer argument for this paper would be clear evidence that \emph{the perception maintainers have of their clients/users/community is often wrong}. Do we have that?! \emph{Javan states that ``developers are much more likely to err on the side of caution when it comes to breaking changes, since restrictive constraints and pinned dependencies are substantially more common than permissive constraints'. When inquiring on why dependency smells are introduced, they find out that, although developers have not directly experienced breaking changes with certain libraries, past experiences make them distrust semver conventions and prevent upgrading to a new release: ``I think it is a result of several incidents with packages and my mistrust of [the] js community'''. These observations can be crossed with our results (EMSE'21), but to be fair we are talking about different ecosystems, with different values and practices.}
	\item The \emph{opportunity} cost of an activity or option is the loss of value or benefit that would be incurred (the cost) by engaging in that activity or choosing that option, versus/relative to engaging in the alternative activity or choosing the alternative option that would offer the highest return in value or benefit:~not making change to be kind to downstream users vs. having to maintain old interfaces, being immobile, \etc
\end{itemize}

% Motivation
\begin{itemize}
	\item Do we have any data or RW that motivates the need for BreakBot? $\rightarrow$ ESEM'21 shows that BCs have a low impact on clients;~Spoon/Coq are already using some kind of ``reverse CI'' but with many problems;~Apache/Guava are concerned about backwards-compatibility and are using tools to signal the introduction of BCs;~\etc
	\item Some RW that would show that developers/maintainers are ``scared'' of making changes in their public APIs?
	\item Can we show a concrete example (a PR on Guava or similar?) that depicts how developers are talking about these problems, and how a bot would assist them in their decisions?
	\item Without tool support, conducting refactoring on your own code is tricky as code size and complexity grows;~imagine the pain of having to understand the impact of your changes on code that you do not even own! (or know about!)
	\item Perhaps describe what happens when a library maintainers receives a PR:~what is he looking for? which health checks? what's the information missing for proper decision making? \etc
\end{itemize}

%Longitudinal study (Build a “tendency to break clients” metric over time to reinforce/deteriorate trust in libraries.)

\subsection{Future Plans}

Our prototype implementation of the vision, \bb, is a mere stepping stone.
For our vision to become a reality and bring the expected benefits, the following research questions must be addressed.

\paragraph{Quantitative evaluation}
\begin{itemize}
	\item Is BreakBot accurate on the detections side? Precision, recall, \etc. Benchmark? Jezek? etc.
\end{itemize}

\paragraph{Qualitative evaluation}
\begin{itemize}
	\item Conduct interviews with maintainers who have already implemented some kind of ``reverse CI'':~why did they do that? what did it change? what are the current pain points? how would BreakBot fit? (\eg Coq, Spoon, Scala, Linux, Apache)
	\item Deploy BreakBot on a selected few libraries and conduct qualitative interviews. Two axes: is the idea of having a BreakBot helpful? is the implementation in BreakBot good? (\eg Spoon, JavaParser, ASM, Vallang, GumTree)
	\item Does it ``scare'' developers more or does it encourage them to make changes they were afraid of?
	\item Interview different ``profiles'':~people who've implemented some kind of reverse CI, people who've implemented BC analysis (\eg with japicmp), people who did not care about it yet
\end{itemize}

\paragraph{Automatic discovery of clients} Coq and Spoon have a precise list of clients they would like to check. This is not the case for everyone. Could we automatically infer the list of clients to check? How can we avoid analyzing the same kind of clients multiple times? How do we cluster them? How do we discard ``uninteresting'' clients? How do we automatically pick the right versions to check? \etc

\paragraph{Configurability} Each ecosystem and library has its own values and policies regarding stability and evolution. Tool support for enforcing these policies must be highly configurable in order to support the users' expectations.

\paragraph{Usage model} Also, we do not currently build a proper \emph{usage model} and rather look in the source code of each client how it's impacted, not how it uses the library to then derive the impact. Maybe that could be a better approach?

\paragraph{Counting detections} Currently, it is still blurry what are the list of BCs, how critical they are, how detections should be reported, \etc What is the semantics of one detection? Currently detection = count every node in the AST impacted by a change; that's not the right abstraction for developers; could it be lines? something else? is it scenario-specific? etc.

\paragraph{Trying to have a report that is closer to developer's intentions}
If a developer renames a method; he loses this information in the report. We should be able to \eg aggregate a set of japicmp BCs to an "intention" of the developer (\eg renaming a method).

\paragraph{Future Work}
There are 
Behavioral evolution;~ecosystem-scale BreakBot;~``tendency to break clients over time'' metric and badge to reinforce trust;~Dependabot-reloaded.

\paragraph{Coccinelle} Don't forget to mention it somewhere, as Julia's in the PC ;) Also, is there some kind of reverse CI for the kernel or its drivers?

%\paragraph{Random idea}
%Can we look at breaking commits according to conventional commits\footnote{\url{https://www.conventionalcommits.org/}} to see if they're actually breaking?
